# Supplementary material for: Holistic 3D Human and Scene Mesh Estimation from Single View Images
Source: arXiv:2012.01591 source file (2021-04-16)
Supplement: Supplementary file 3 [file quali_high_res.pdf]

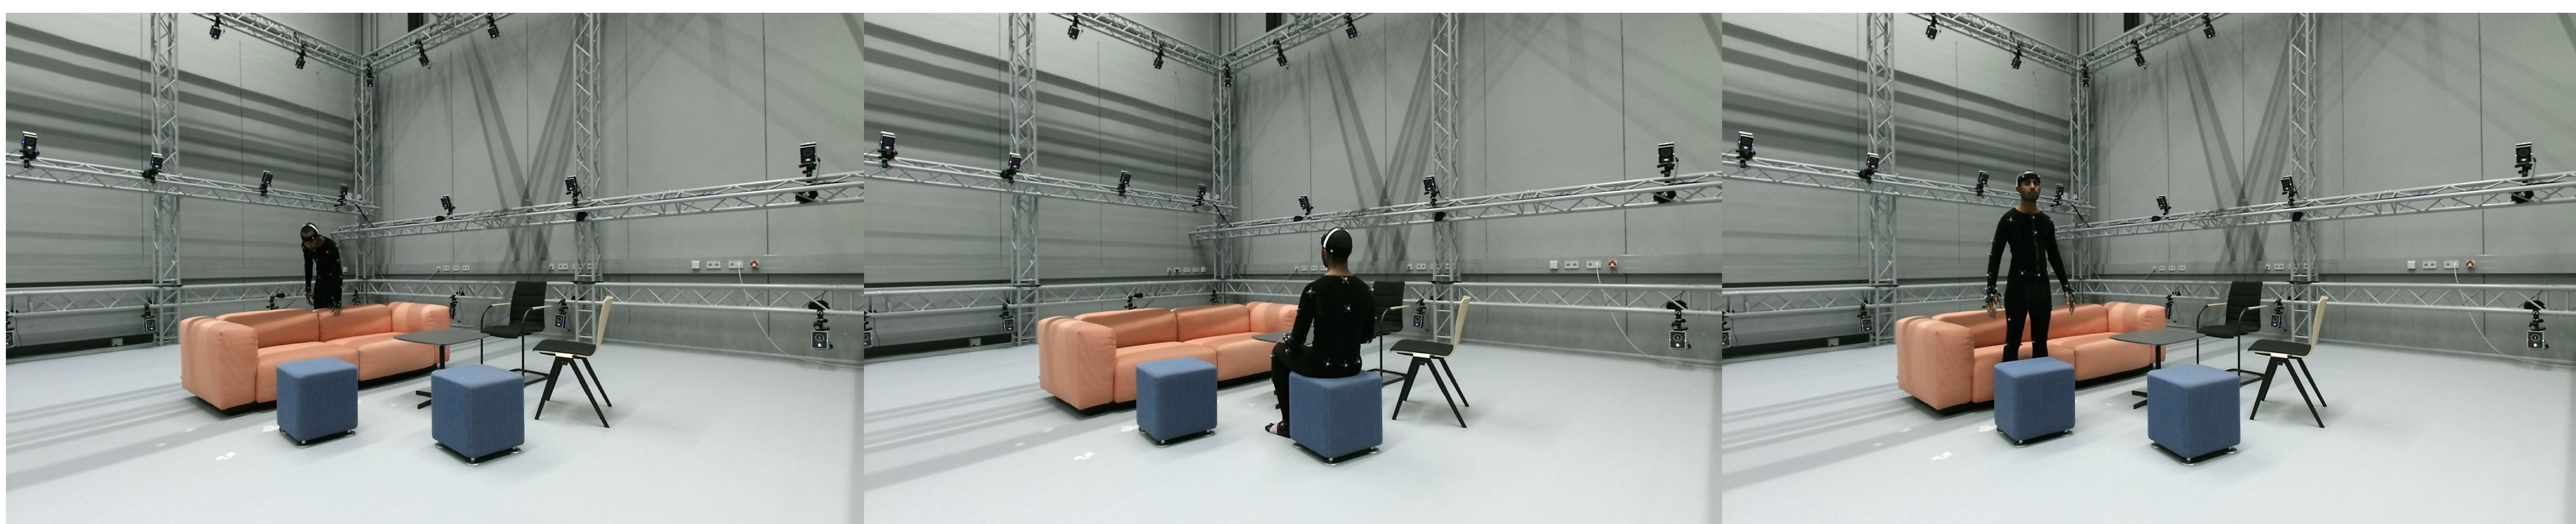

RGB input

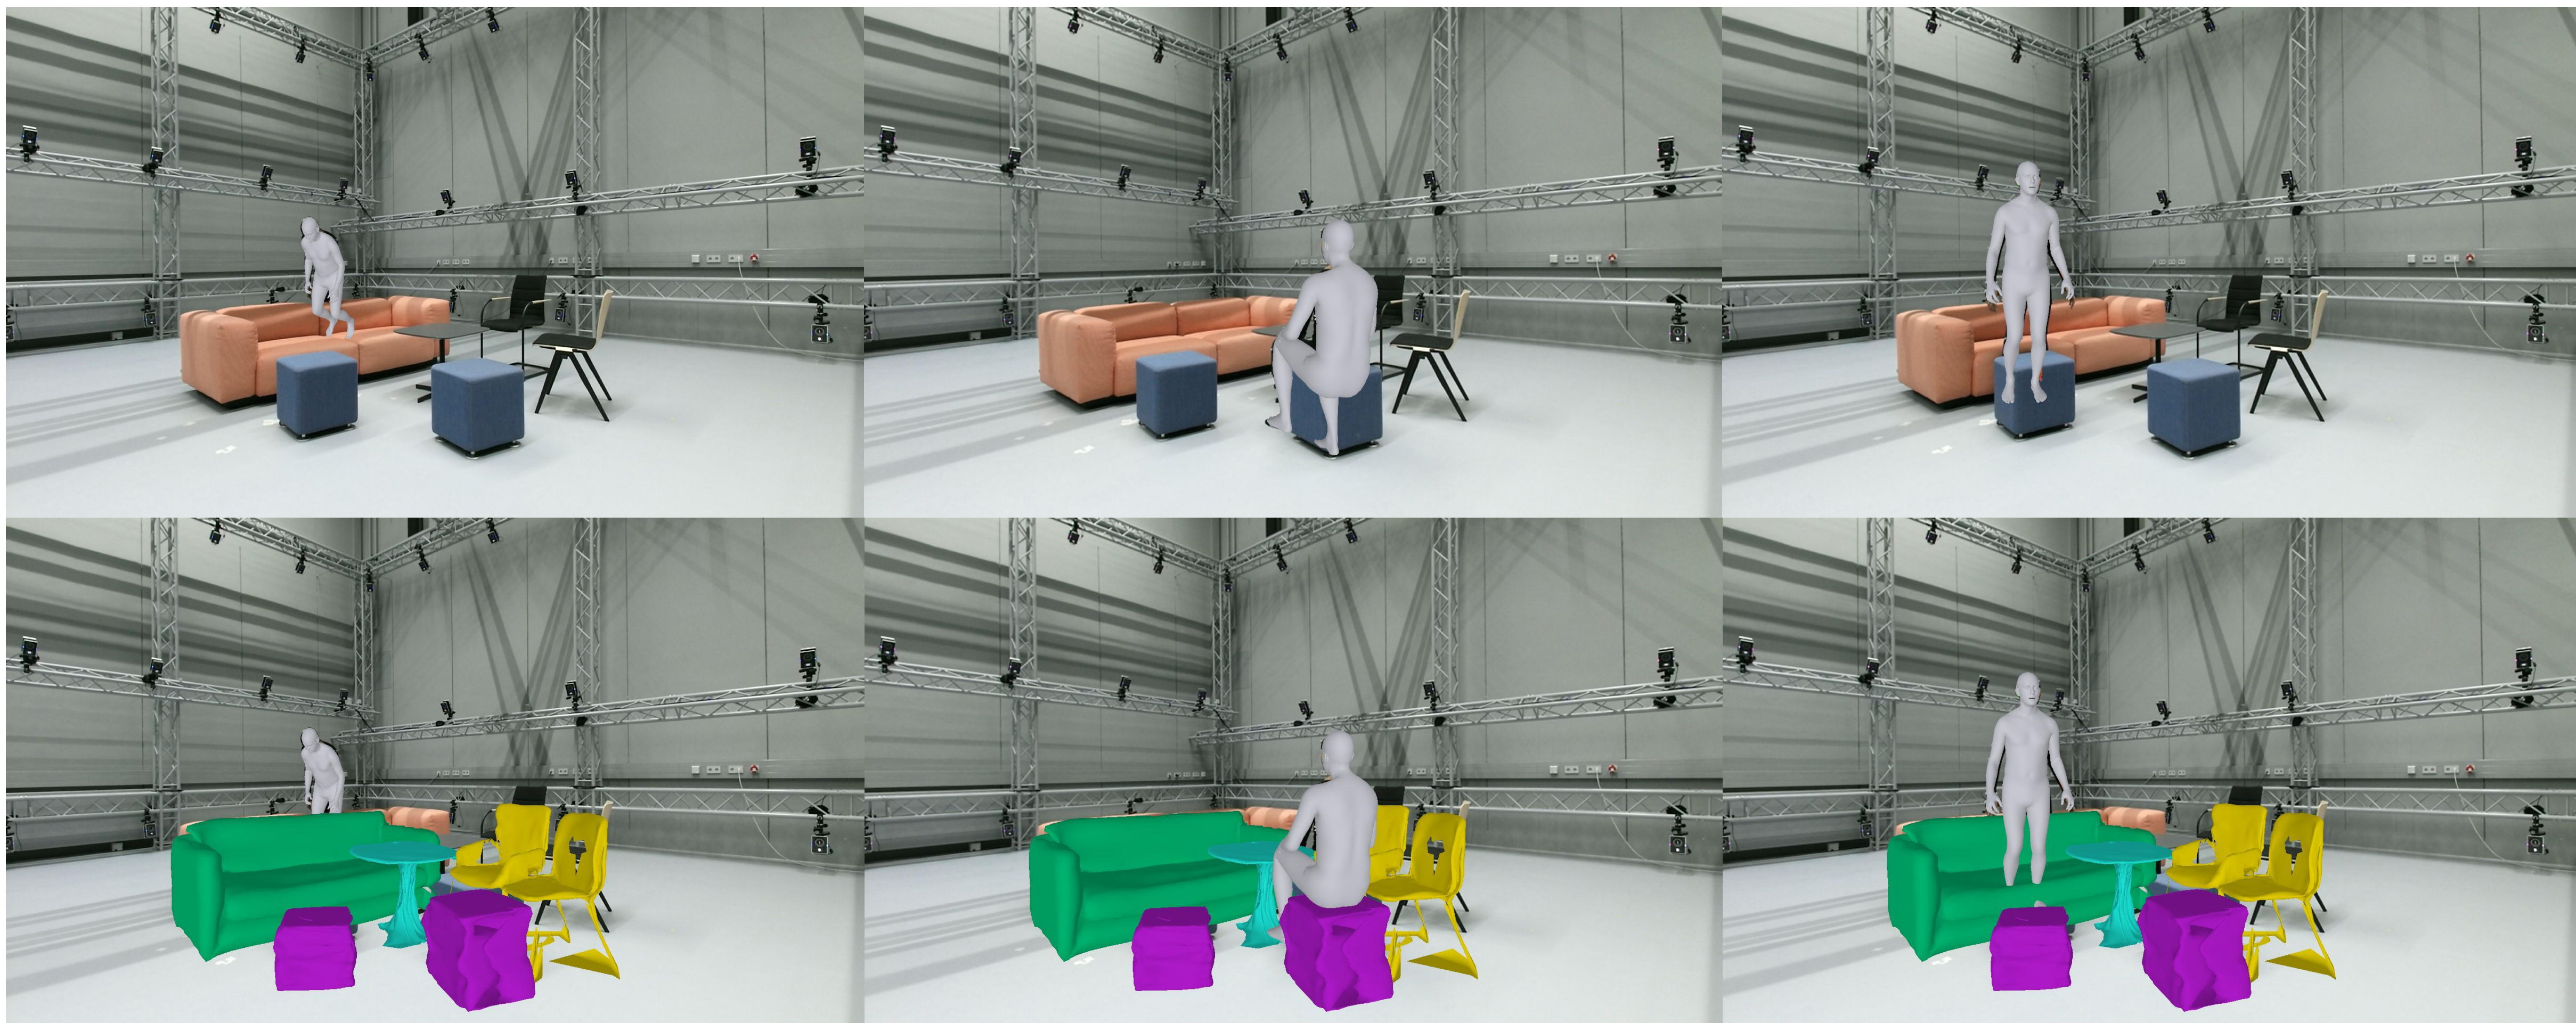

Initial body mesh (shown together with final scene mesh in lower row)

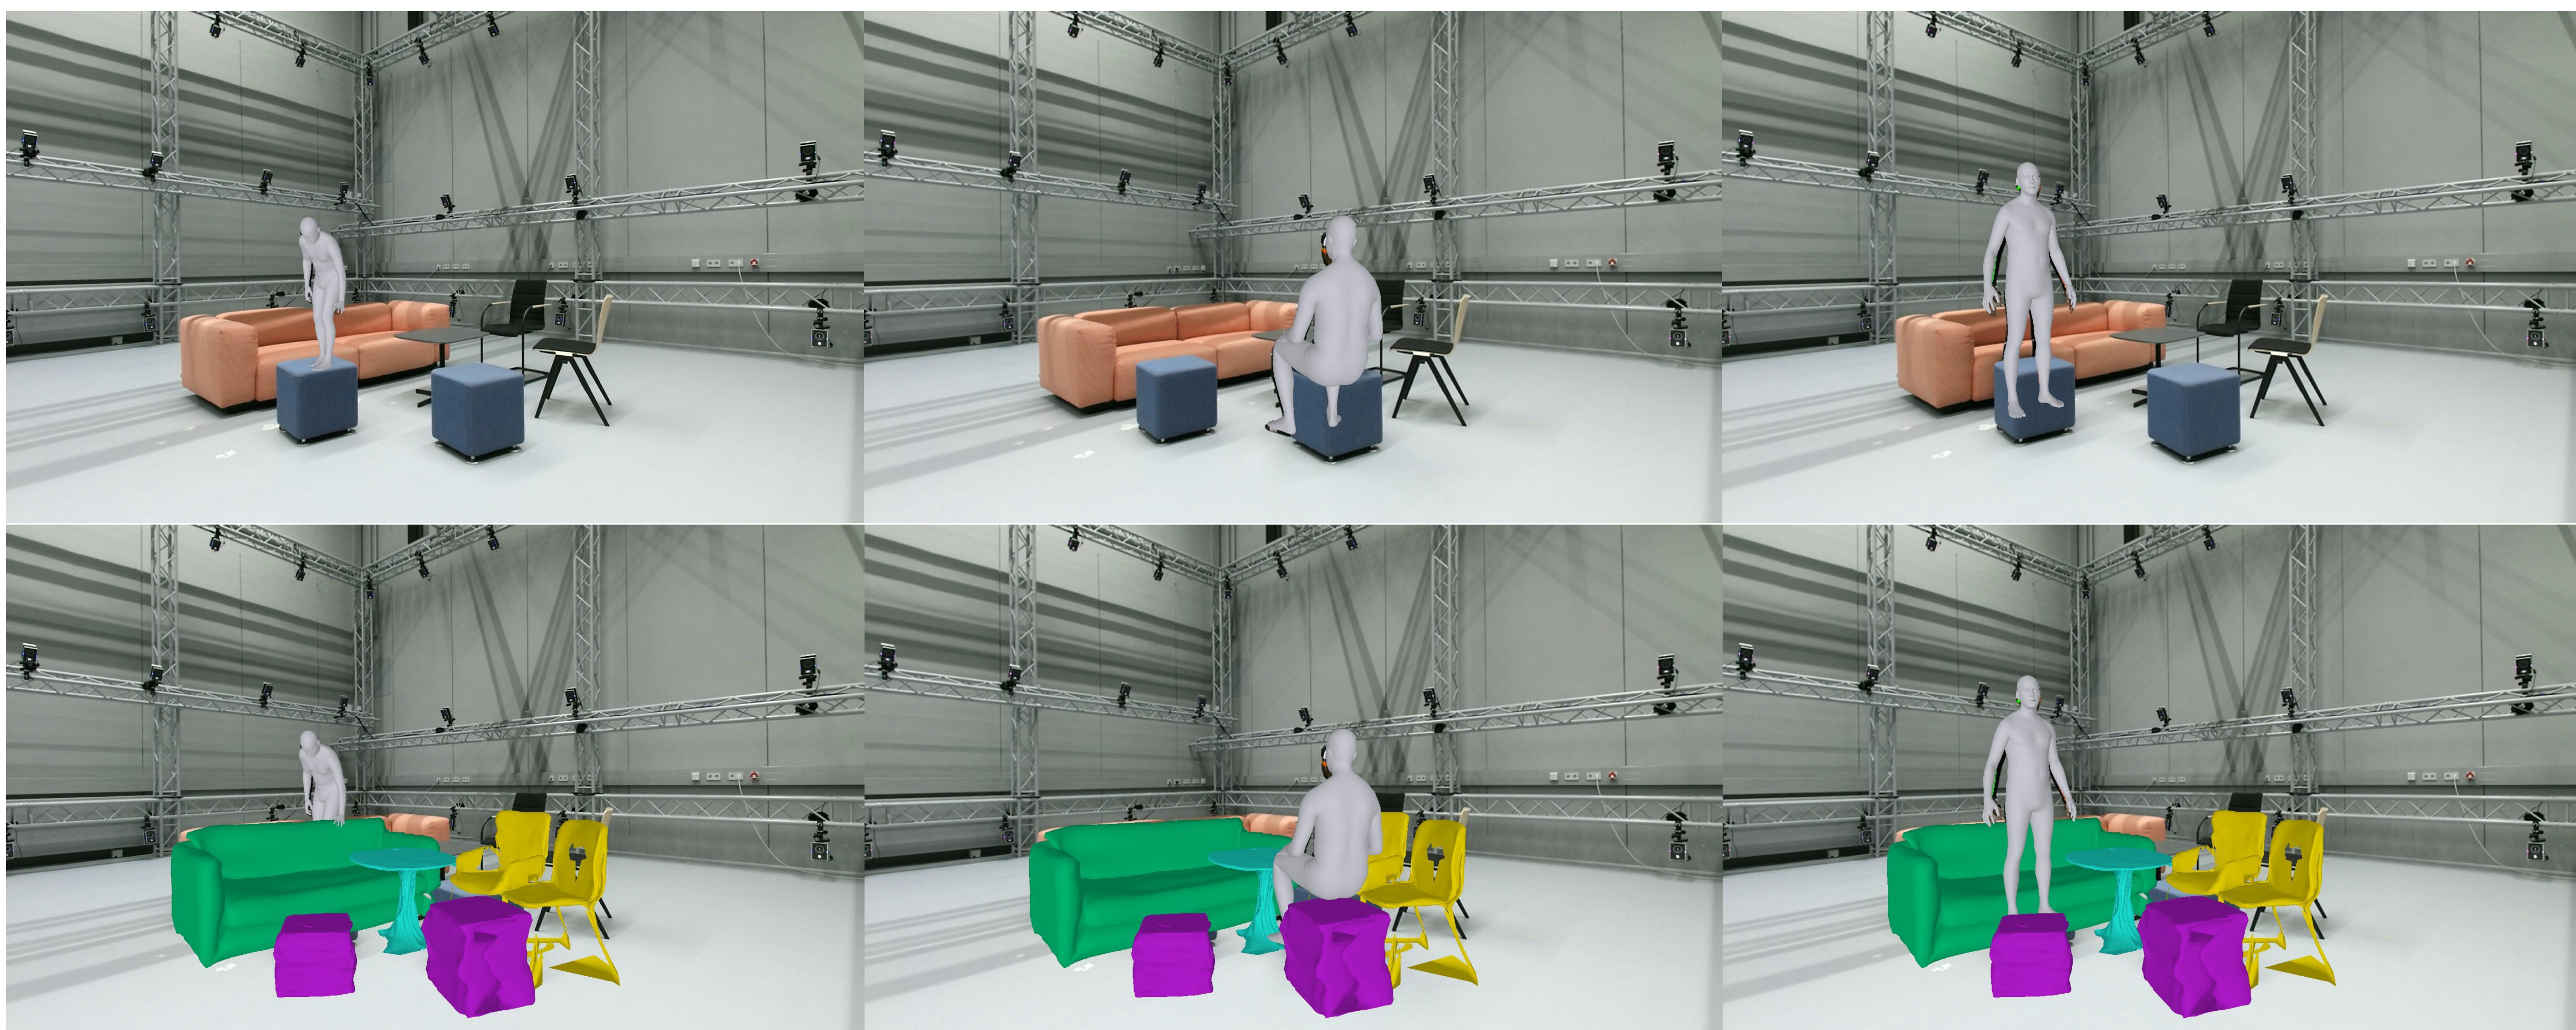

Final body mesh (shown together with final scene mesh in lower row)

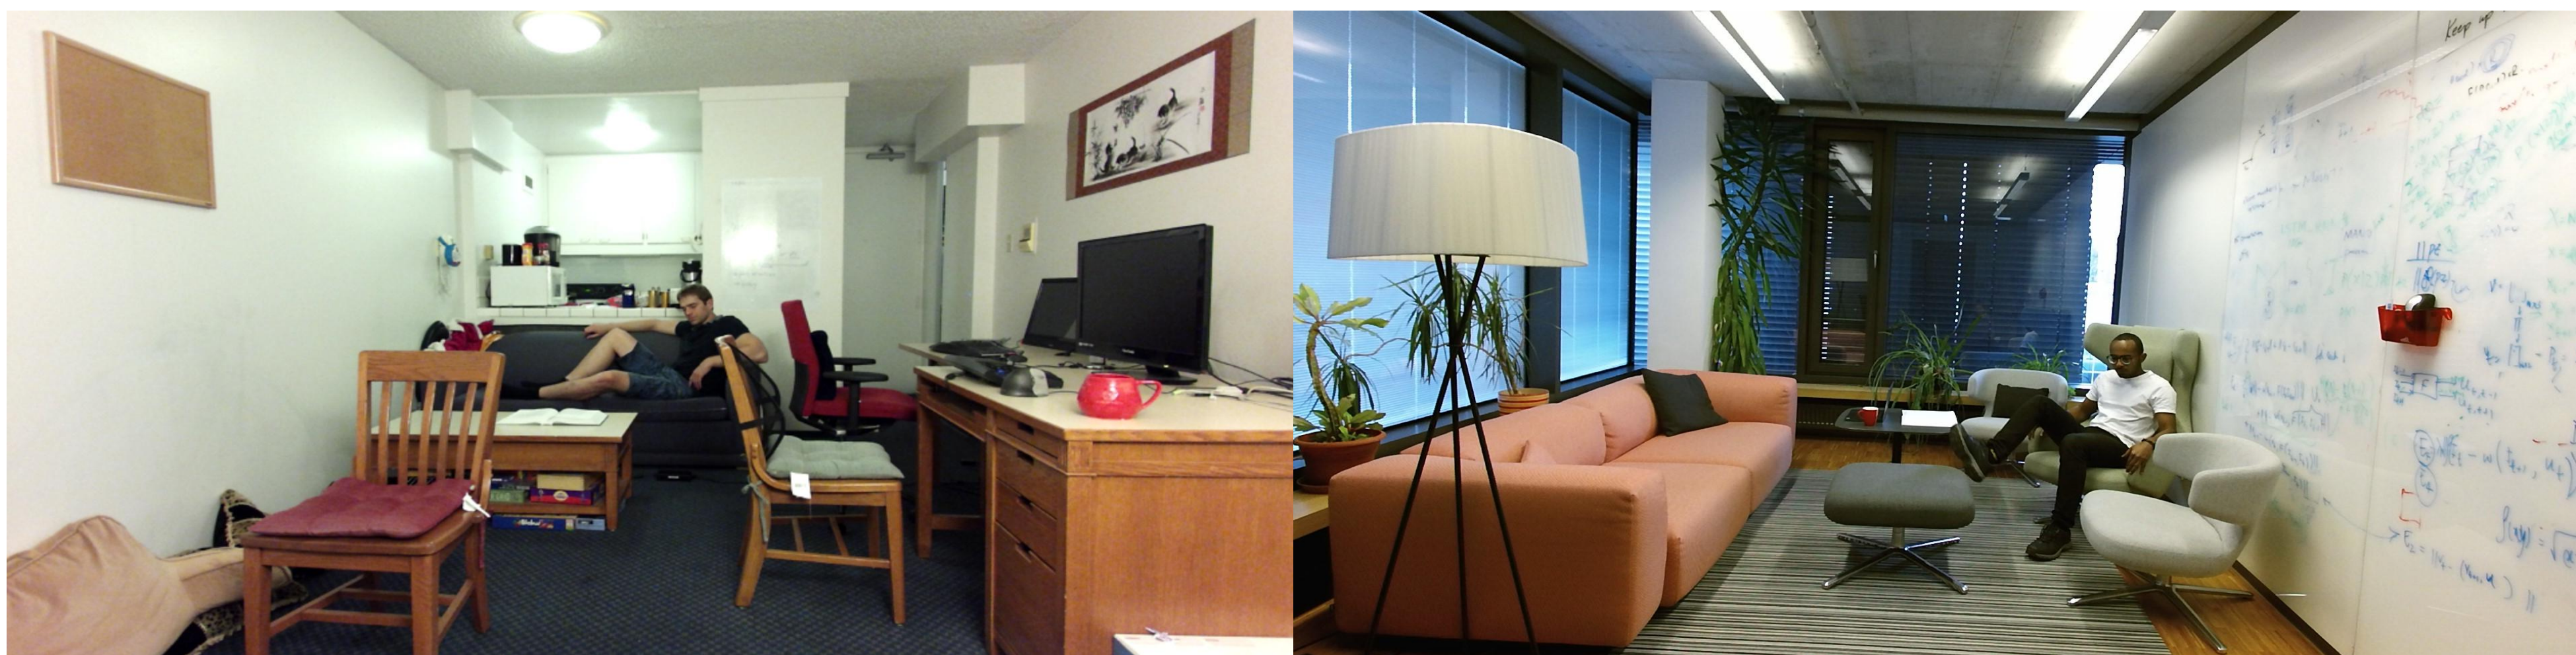

RGB Input

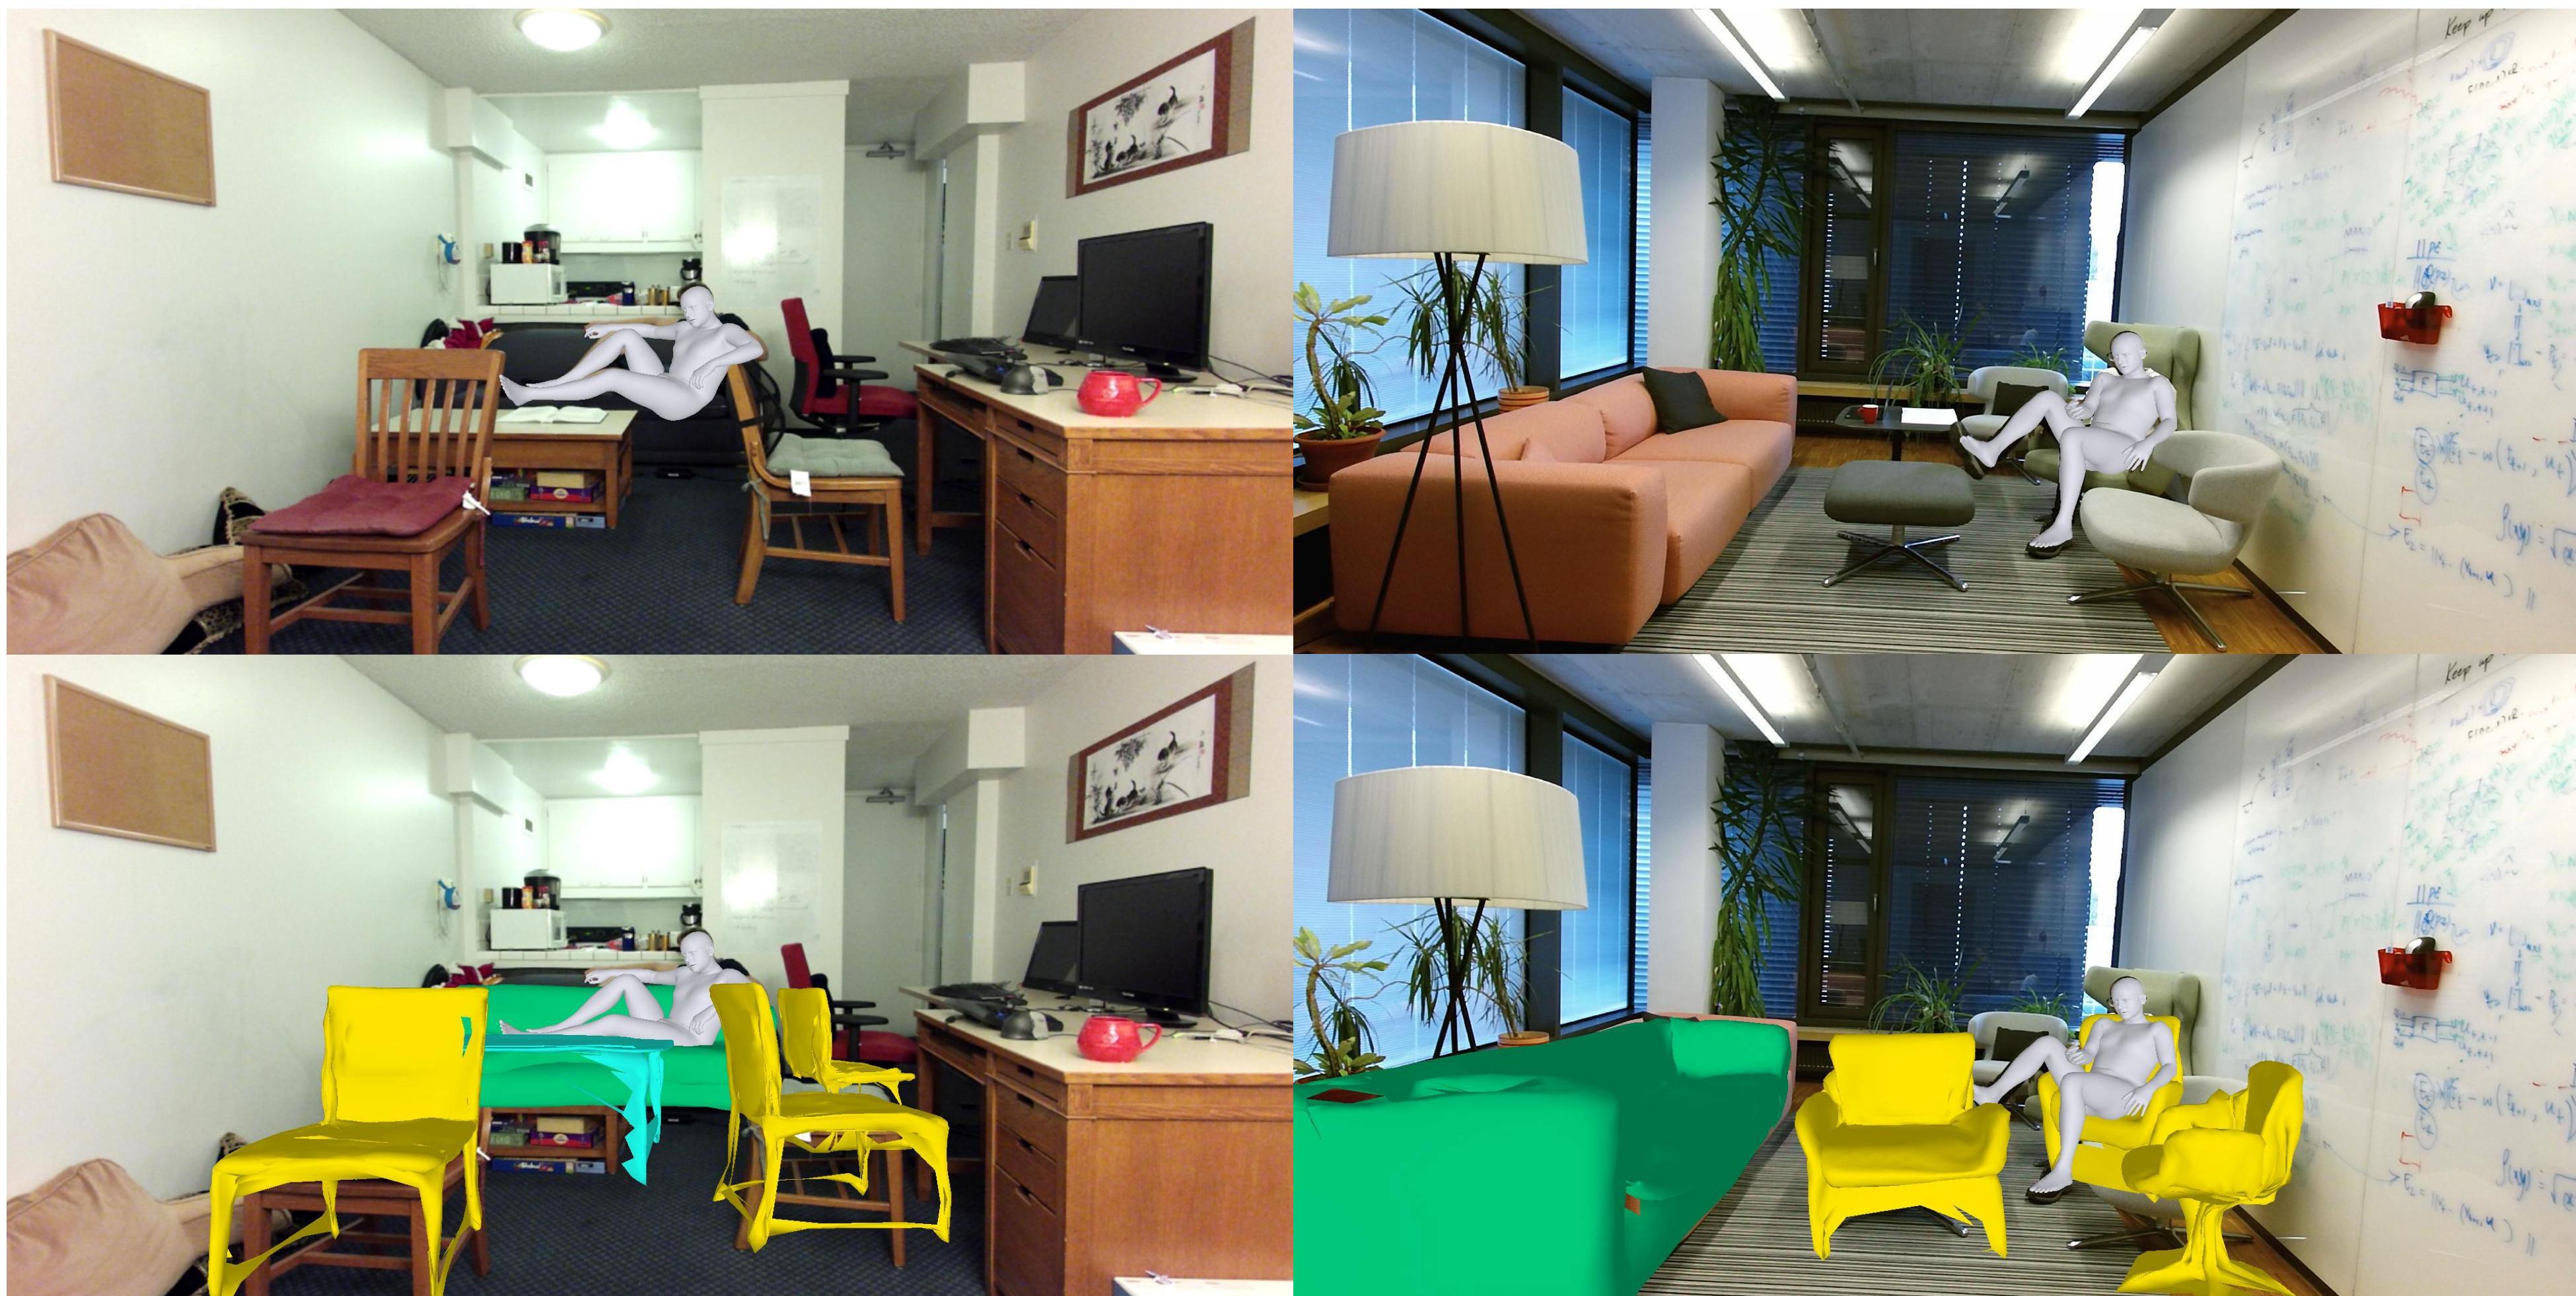

Initial body mesh (shown together with final scene mesh in lower row)

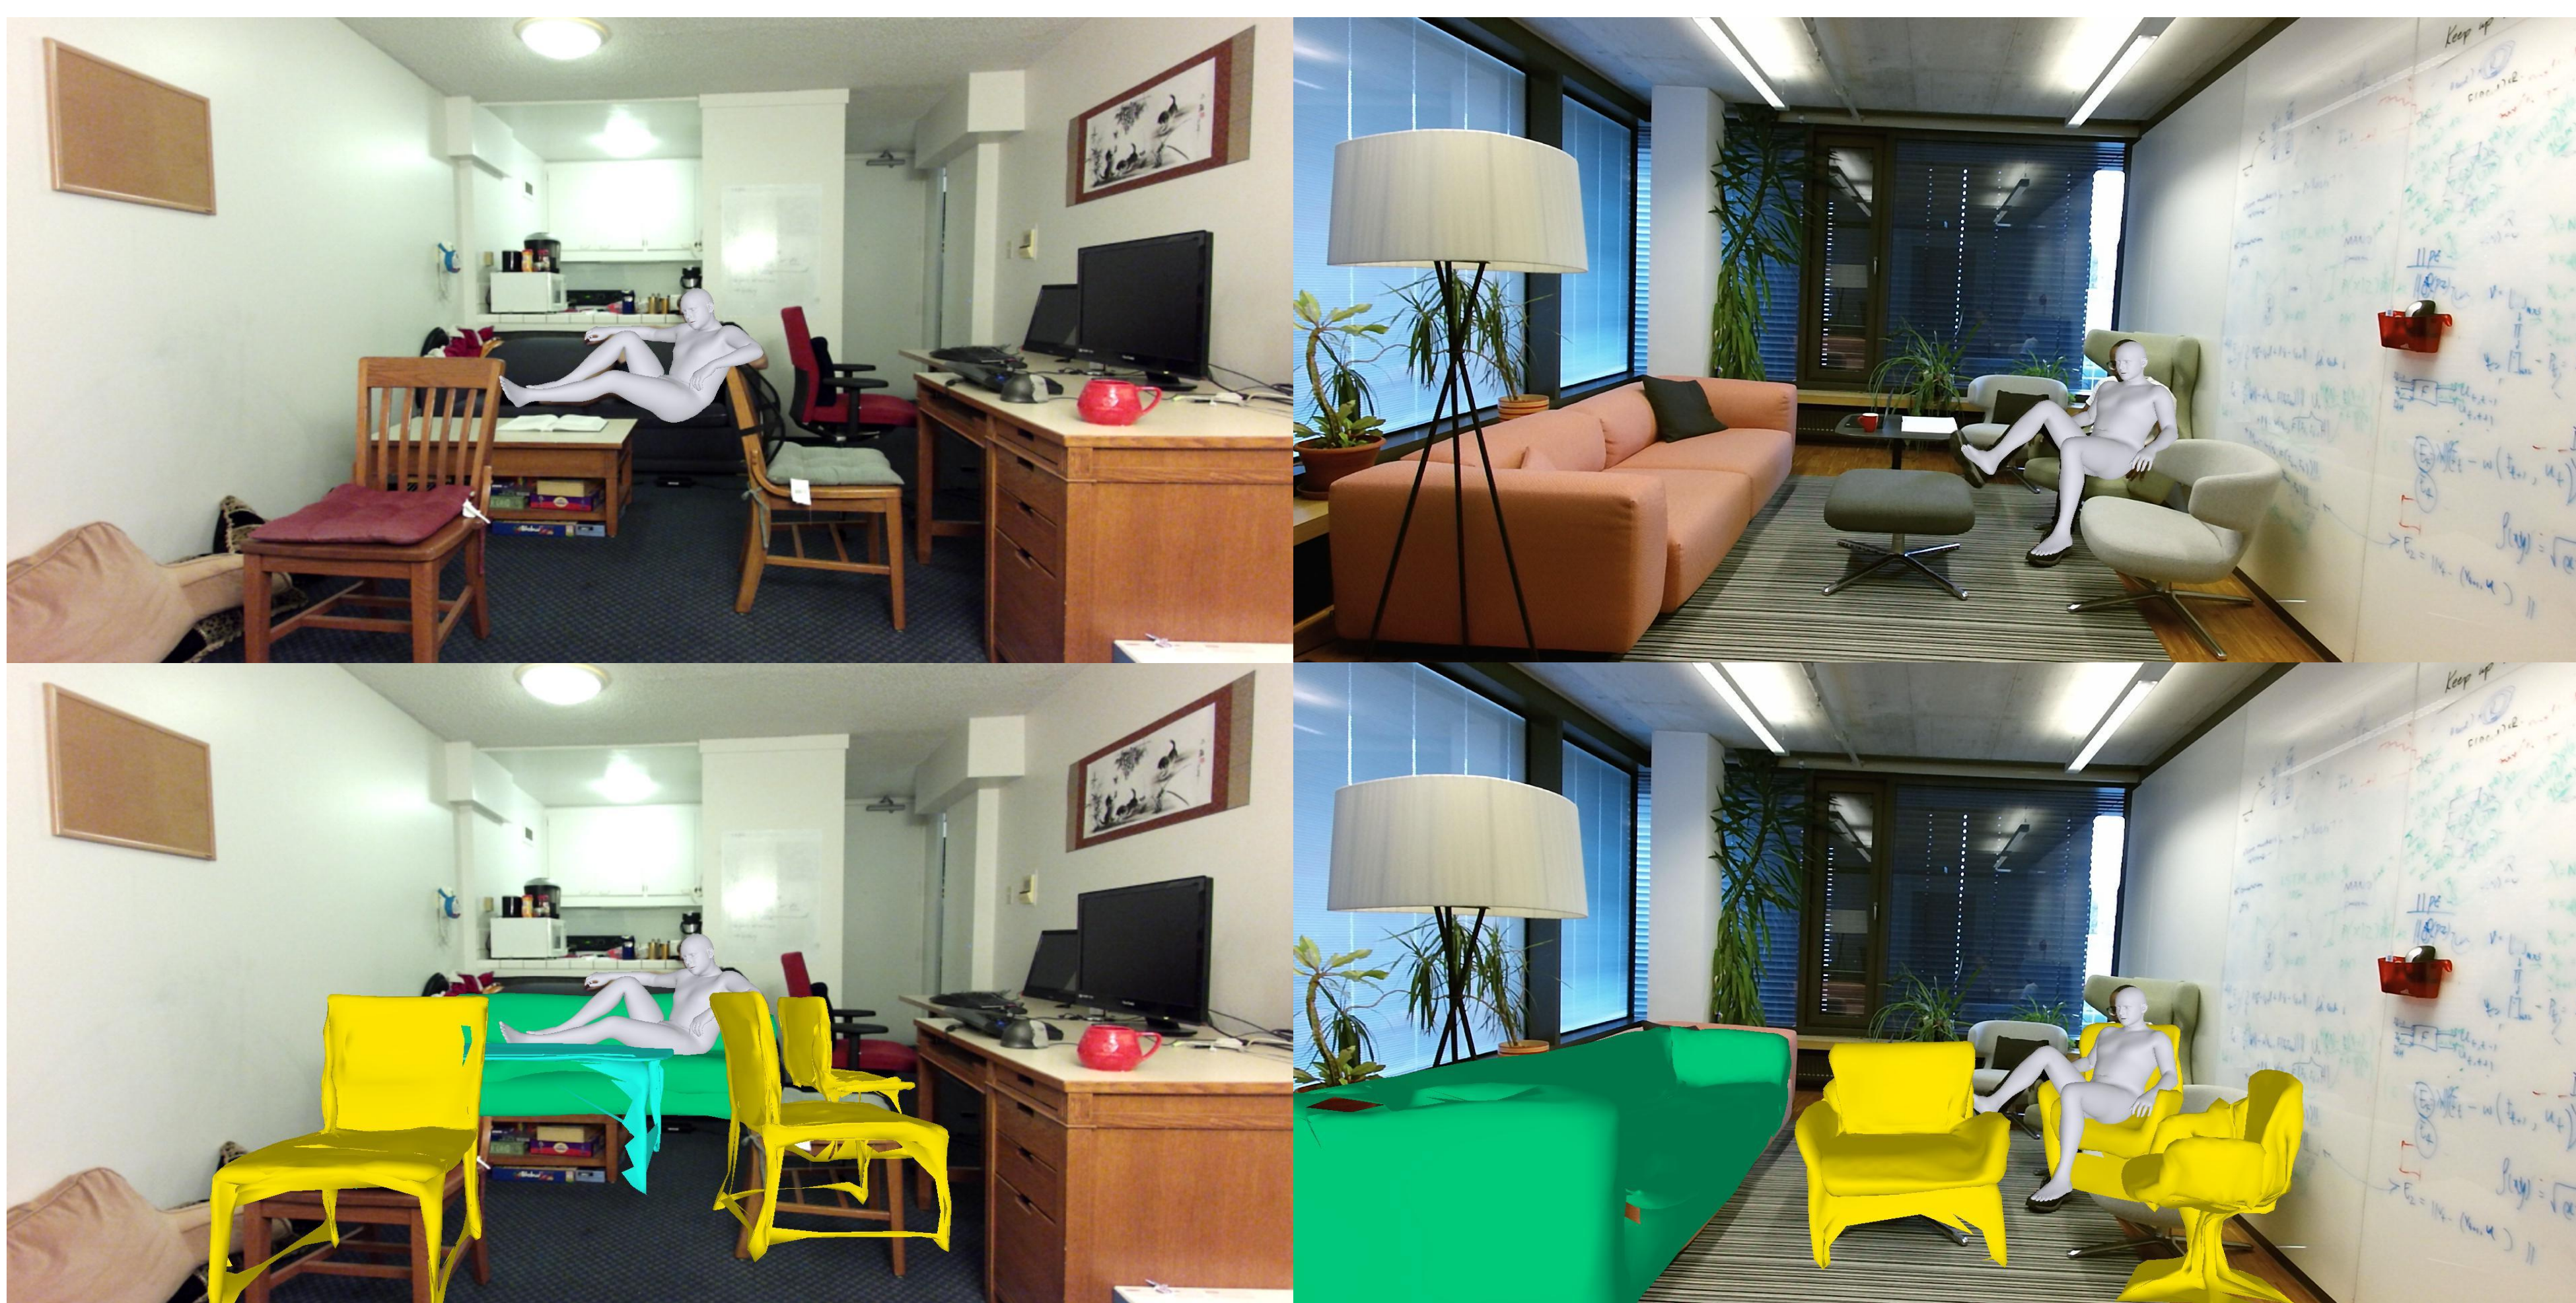

Final body mesh (shown together with final scene mesh in lower row)
